# Supplementary material for: AXNav: Replaying Accessibility Tests from Natural Language
Source: arXiv:2310.02424 source file (2024-03-05)
Supplement: Supplementary file 1 [file 9_appendix.tex]

\section{Appendix}
\label{section:appendix}

\subsection{Formative Study Interview Questions}
\begin{itemize}
    \item What are some of the challenges of manual testing for accessibility?
    \item Have you ever done any manual testing of app accessibility? Give me an example.
    \item When do you conduct manual accessibility testing?
    \item Have you ever written down any instructions to instruct others how to test your app’s accessibility manually (Manual tests for QA)? If so, how do you write them? What level of detail do you include?
    \item What are some of the areas and features you test your app’s accessibility (manually) for? 
        \begin{itemize}
            \item Pick an app (that you’ve worked on or tested) on your phone and demonstrate how you test the feature. Please think aloud while you are testing and show what you are doing. 
        \end{itemize}
    \item How do you know whether your test succeeds or fails? 
    \item If you could speak / write down a high-level description and an accessibility feature you want to test, and a tool could replay the instructions on a device to demonstrate the test, what would be your reaction to this?
        \begin{itemize}
            \item (First, show them input accessibility test instructions, taken from a real regression testing database of manual AX tests. Then show them a screen recording of the test being performed manually on a mobile phone by an author. Ask to imagine the system is replaying the instructions on the device). 
            \item What features should this tool support? 
            \item Would there be any benefits or drawbacks you can think of to have this functionality?
            \item Would you use this in your testing workflow? Why or why not? If yes, how might you use it? 
        \end{itemize}
\end{itemize}

\subsection{Test Instructions Used to Generate Videos for User Study}
\begin{itemize}
    \item Title: iOS: Media App: VoiceOver: Share an Episode; Instructions: iOS: Media App: VoiceOver: Share an Episode 
    \item Title: iOS: Large Text in Following Tab
    \item Title: iOS: Media App: Button Shapes across app; Instruction: iOS: Media App: Button Shapes across app; Expected Results: When Testing button shapes - we want to make sure that all text (not emojis or glyphs) get underlined if they are NOT inside of a button shape already. If the text is already within a button shape, it is a bug! (We see this bug frequently) 
\end{itemize}

\subsection{User Study Interview Questions}
For each video demo: 

\begin{itemize}
    \item Please think out loud when you are going through the video.
    \item Do you want to replay the video or scrub through certain parts? You can also use the chapters to navigate
    \item What is your first reaction after seeing the video? Did the test go as you expected? Why or why not? Are there any parts that you found surprising? Are there any steps that were missed or went wrong?
    \item How similar or different is this from what you might do to test this manually? On a scale of 1-5, rate how well this test video replicates how you might perform this test manually. Please explain your answer (5 - Extremely good match, 4 - Very good match, 3 - Moderately good match, 2 - Slightly matches, 1 - Not at all) 
    \item What do you think about the similarities/differences? 
    \item Did you find any issues or bugs in the video? How serious is this issue? If this is a real issue you found, would you file an internal bug report for this? Why or why not?
    \item How did the heuristics for flagging issues assist with that? Please rate and explain your answer. (5 - Very useful, 4 - Useful, 3 - Moderately useful, 2 - Somewhat useful, 1 - Not useful at all)
    \item How can the heuristics be improved? 
\end{itemize}
 
General reflection:  

\begin{itemize}
    \item How do you imagine using this system in your existing practice?
    \item If the system was able to replicate these tests extremely well, how useful might it be in your existing work? Please rate and explain your answer. (5 - Very useful, 4 - Useful, 3 - Moderately useful, 2 - Somewhat useful, 1 - Not useful at all)
    \item How useful would the system be to your work in its current form today? Please rate and explain your answer. (5 - Very useful, 4 - Useful, 3 - Moderately useful, 2 - Somewhat useful, 1 - Not useful at all)
    \item What drawbacks or benefits can you think of for this system?
    \item What other accessibility test types would you like the system to support? 
    \item What other use cases related to accessibility can you imagine for this system?
    \item What other features would you like the system to have?
\end{itemize}

\subsection{Participants information}

The profiles of our participants are listed in Table \ref{table:userstudy-participants}.
% Please add the following required packages to your document preamble:
% \usepackage[table,xcdraw]{xcolor}
% If you use beamer only pass "xcolor=table" option, i.e. \documentclass[xcolor=table]{beamer}
\begin{table*}[h]
\begin{tabular}{l llll}
\textbf{Participant ID} & \textbf{Order of videos} & \textbf{Gender} & \textbf{Accessibility tasks in job duty}                                                                                                                                  & \textbf{Years of experience} \\
\textbf{P1}                                     & BS, DT, VO                                       & M                                       & \begin{tabular}[c]{@{}l@{}}Manual accessibility testing; \\ QA testing for accessibility; \\ Writing accessibility automation tests\end{tabular}                                                  & 3                                                    \\
\textbf{P2}                                     & DT, VO, BS                                       & M                                       & \begin{tabular}[c]{@{}l@{}}Designing or building accessibility features; \\ Manual accessibility testing; \\ QA testing for accessibility\end{tabular}                                            & 4                                                    \\
\textbf{P3}                                     & BS, VO, DT                                       &                                         &                                                                                                                                                                                                   &                                                      \\
\textbf{P4}                                     & VO, DT, BS                                       & F                                       & Writing accessibility automation tests                                                                                                                                                            & 6                                                    \\
\textbf{P5}                                     & BS, DT, VO                                       & F                                       & \begin{tabular}[c]{@{}l@{}}Designing or building accessibility features; \\ Manual accessibility testing\end{tabular}                                                                             & 3                                                    \\
\textbf{P6}                                     & DT, BS, VO                                       & F                                       & \begin{tabular}[c]{@{}l@{}}Manual accessibility testing; \\ QA testing for accessibility\end{tabular}                                                                                             & 3                                                    \\
\textbf{P7}                                     & VO, BS, DT                                       & M                                       & Designing or building accessibility features                                                                                                                                                      & 6                                                    \\
\textbf{P8}                                     & DT, VO, BS                                       & M                                       & \begin{tabular}[c]{@{}l@{}}Designing or building accessibility features; \\ Manual accessibility testing; \\ QA testing for accessibility; \\ Writing accessibility automation tests\end{tabular} & 9                                                    \\
\textbf{P9 (P4 in formative study) }                                     & VO, BS, DT                                       & M                                       & \begin{tabular}[c]{@{}l@{}}Designing or building accessibility features; \\ Manual accessibility testing; \\ QA testing for accessibility\end{tabular}                                            & 4                                                    \\
\textbf{P10 (P5 in formative study)}                                    & DT, BS, VO                                       & F                                        & \begin{tabular}[c]{@{}l@{}}Manual accessibility testing; \\ QA testing for accessibility; \\ Writing accessibility automation tests\end{tabular}                                                                                                                                                                                                  & 2                                                    
\end{tabular}
    \caption{Participants in the user study.}
\label{table:userstudy-participants}
\end{table*}
